# Supplementary material for: Advances in Constraining Intrinsic Alignment Models with Hydrodynamic Simulations
Source: arXiv:2009.10735 source file (2020-09-22)
Supplement: Supplementary file 1 [file appendix4.tex]

In the main body of this work, when we fit the more complicated
TATT model, we use fiduical flat priors on its parameters.
That is, $A_1=[-6,6]$, $A_2=[-6,6]$, $b_{\rm TA} = [0,8]$.
The latter is informed by the idea that the matter - galaxy tidal field
coupling should be equivalent to the galaxy bias on linear scales.
In practice, the situation may be more complicated than this. 
We note that in all cases where $b_{\rm TA}$ is meaningfully constrained, 
the posteriors are at least partly cut off by the lower edge of the prior.

To test the impact of the choice of priors, then, we rerun our most constraining
analysis with expanded prior edges. The new priors for this exercise are
$A_1=[-6,6]$, $A_2=[-6,6]$, $b_{\rm TA} = [-8,8]$ 
(the $A_1$, $A_2$ priors are unchanged because the posteriors are always well 
clear of the prior edges for these parameters).
The results are shown in Figure \ref{fig:app:bta_prior}. 
Although the difference is not inperceptible, it does not change our
conclusions; $A_2$ is still consistent with zero, and the centering of the 
$A_1$ constraint is not particularly shifted. 
It is also worth noting that the $b_{\rm TA}$ posterior is centered
on zero, such that the model appears to favour the pure NLA paradigm
above any more complicated scenarios.    

\begin{figure}
\includegraphics[width=\columnwidth]{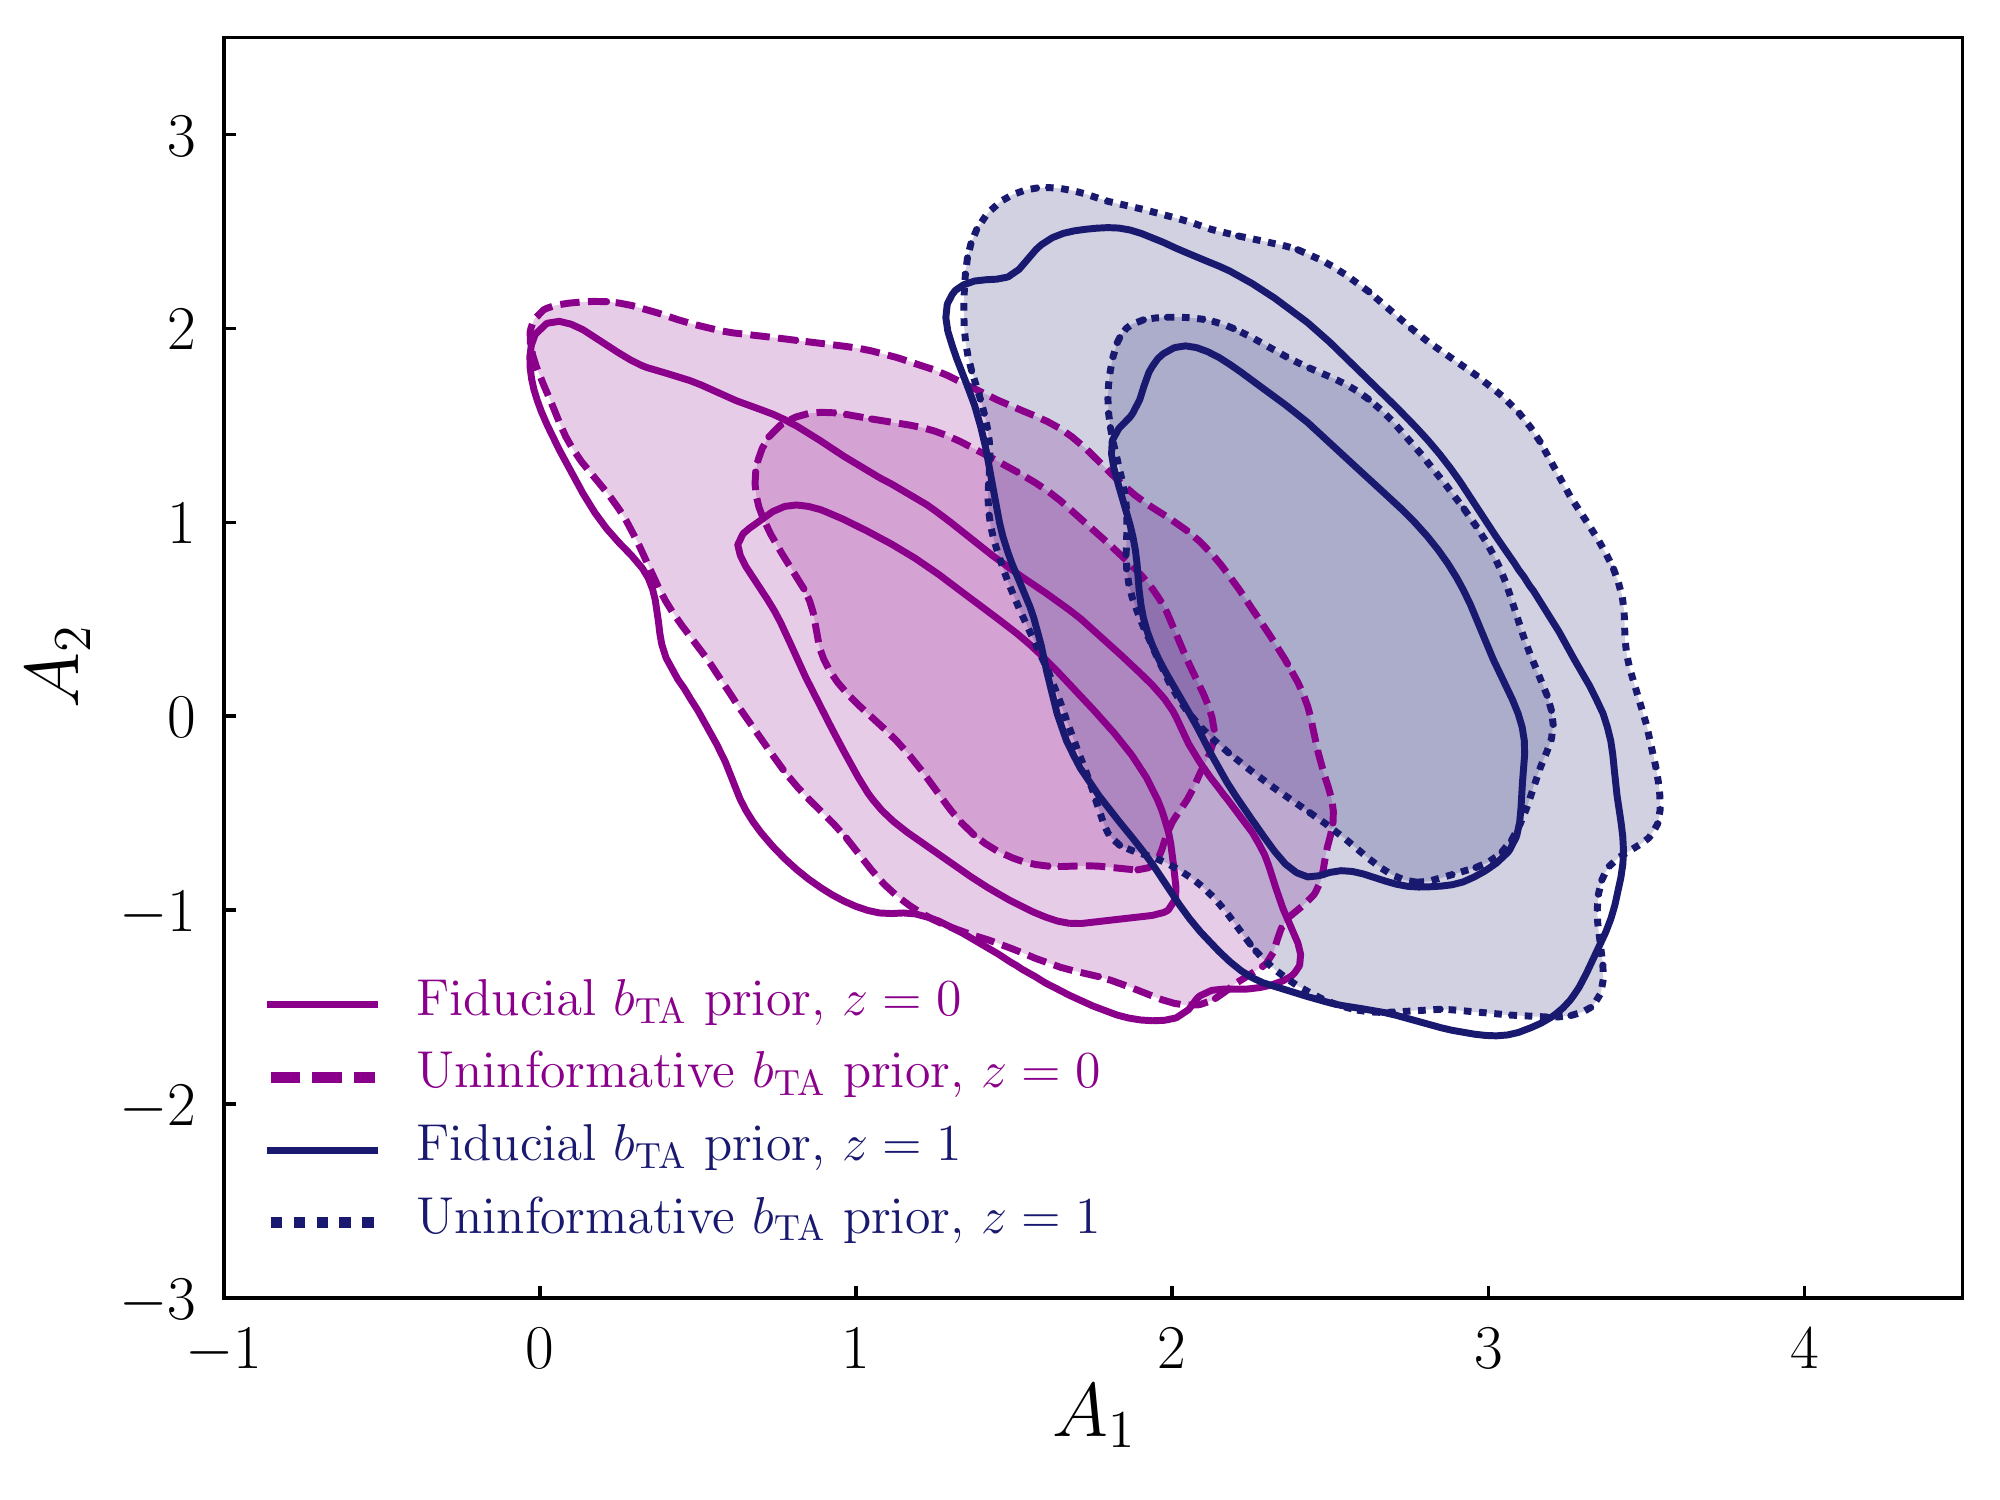}
\includegraphics[width=\columnwidth]{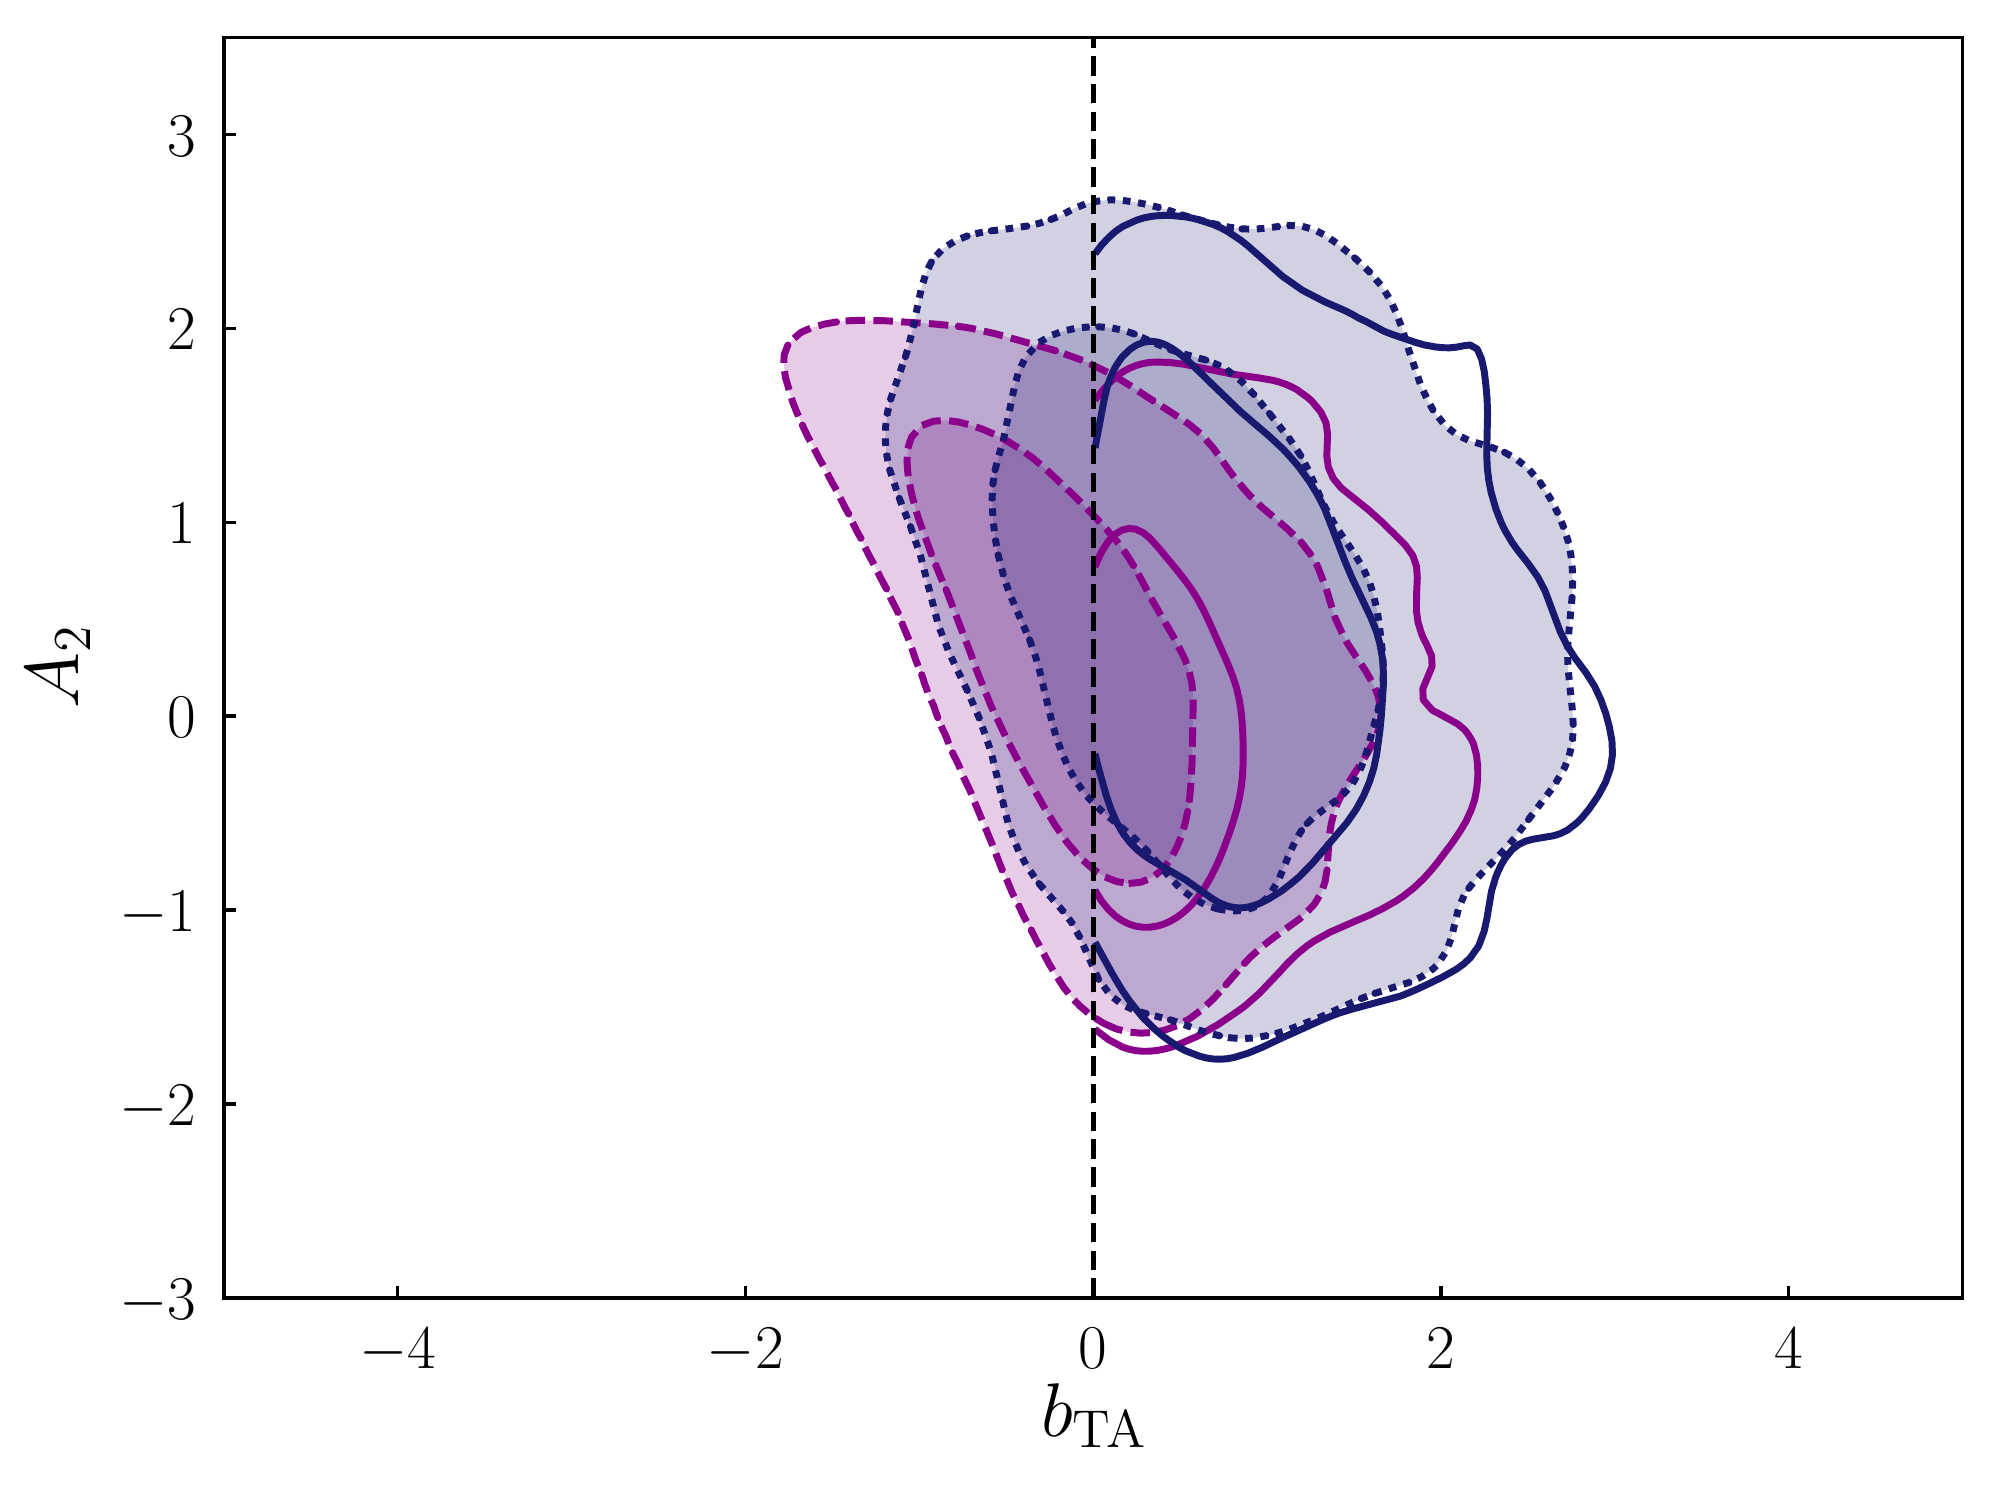}
\caption{The impact of widening the priors on TATT model IA parameters. For illustrative 
purposes we show only the upper and lower-most TNG snapshots here.
In the lower panel the dashed vertical line shows the lower edge of the fiduical 
flat prior on $b_{\rm TA}$.
}\label{fig:app:bta_prior}
\end{figure}
